# Supplementary material for: Dielectric dependent hybrid functionals for heterogeneous materials
Source: arXiv:1901.00824 source file (2019-05-20)
Supplement: Supplementary file 1 [file localhybrid_si.pdf]

# Supplemental Material for “Dielectric dependent hybrid functionals for heterogeneous materials”

Huihuo Zheng*
*Argonne Leadership Computing Facility, Argonne National Laboratory, Lemont, IL 60439, USA*

Marco Govoni†
*Materials Science Division, Argonne National Laboratory, Lemont, IL 60439, USA and*
*Institute for Molecular Engineering, University of Chicago, Chicago, IL 60637, USA*

Giulia Galli‡
*Materials Science Division, Argonne National Laboratory, Lemont, IL 60439, USA and*
*Institute for Molecular Engineering and Department of Chemistry, University of Chicago, Chicago, IL 60637, USA*
(Dated: May 18, 2019)

## I. SETUP OF DENSITY FUNCTIONAL CALCULATIONS

In all of our calculations we used ONCV pseudopotentials [1–3], with a plane-wave cutoff of 70 Rydberg. The structure of $(SiC)_{256}$ is from Ref. [4]; the structures of the H-Si/$H_2O$, CH3-Si/$H_2O$, COOH-Si/$H_2O$ slabs are from Ref. [5] and that of the Si/$Si_3N_4$ interface is from Ref. [6]; the supercells of h-BN and $MoS_2$ were constructed from primary cell structures taken from the Materials Project database [7] (Materials ID: mp-984, mp-2816).

## II. DISENTANGLEMENT OF THE DIELECTRIC PROPERTIES OF INTERFACES

In the main text, we used bisection techniques to build a set of local basis functions $\mathcal{F}$ [Eq. (5)] from the eigenvectors of the dielectric response of slabs representing interfaces. We represented $\bar{\chi}^0$ using the basis set $\mathcal{F}$ (see Eq. 5 in the main text), and we showed that the response of the whole system can be disentangled into contributions from the subsystems:

$$\mathrm{eig}(\bar{\chi}^0_A) \cup \mathrm{eig}(\bar{\chi}^0_B) \cup \mathrm{eig}(\bar{\chi}^0_I) \simeq \mathrm{eig}(\bar{\chi}^0)\,. \tag{S1}$$

Here, we further demonstrate that in the case of silicon/water interfaces the dielectric spectra of the subsystems composing the interface are weakly dependent on their respective environments; to so we compare the eigenvalues of $\bar{\chi}^0_A$ and $\bar{\chi}^0_B$ (see main text, Eq.2 and Fig.4) with those of $\bar{\chi}^0_{A/vacuum}$ and $\bar{\chi}^0_{B/vacuum}$, in which A and B are interfaced with vacuum. It is seen from Fig. S1 that the eigen-spectra of silicon and water when interfaced with each other are close to those of silicon and water interfaced with vacuum, with small differences in the low eigenvalue regions. Note that no covalent bonds are present between the subsystems analyzed here.

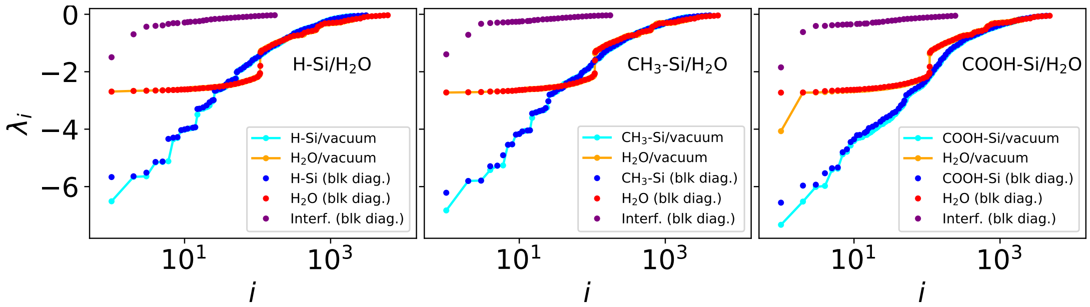


FIG. S 1. Disentanglement of the dielectric spectra of Si/$H_2O$ interfaces (see Eq.2 and Fig.4 in the main text). The eigenvalues of the subsystems (dots) are compared with those of isolated subsystems (Si/vacuum, $H_2O$/vacuum).

* huihuo.zheng@anl.gov
† mgovoni@anl.gov
‡ gagalli@uchicago.edu

## III. LOCAL DIELECTRIC FUNCTIONS

Fig. S2 show the dielectric function $\epsilon(z)$ (average of $\epsilon(\boldsymbol{r})$ over xy planes) of 3D solids (SiC and Si), computed self-consistently using the finite field approach presented in the main text. It is seen that $\epsilon(z)$ shows an atomic scale oscillation (3-5 Bohr) in the 3D bulk. The calculations are converged within 2-3 iterations.

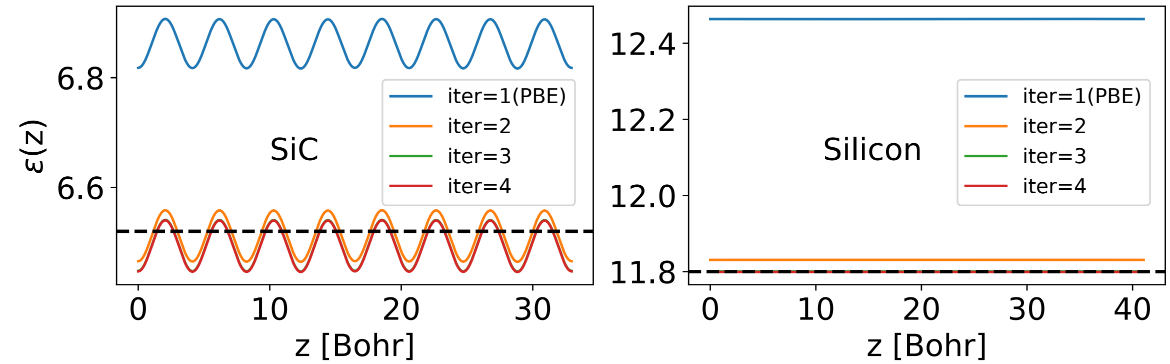


FIG. S 2. Local dielectric function $\epsilon(\boldsymbol{z})$ for SiC and Si. The ionic coordinates are fixed and there is no contribution from ionic displacements. Dashed curves are experimental values of $\epsilon_\infty$ [8].

Fig. S3 shows the $\epsilon(z)$ of 2D materials, $MoS_2$ and h-BN. The spread of $\epsilon(z)$ provides a quantitative measure of the "dielectric thickness" of a 2D monolayer. It is seen that the spread of $\epsilon(z)$ is slightly larger than that of $\rho(z)$ – the charge density.

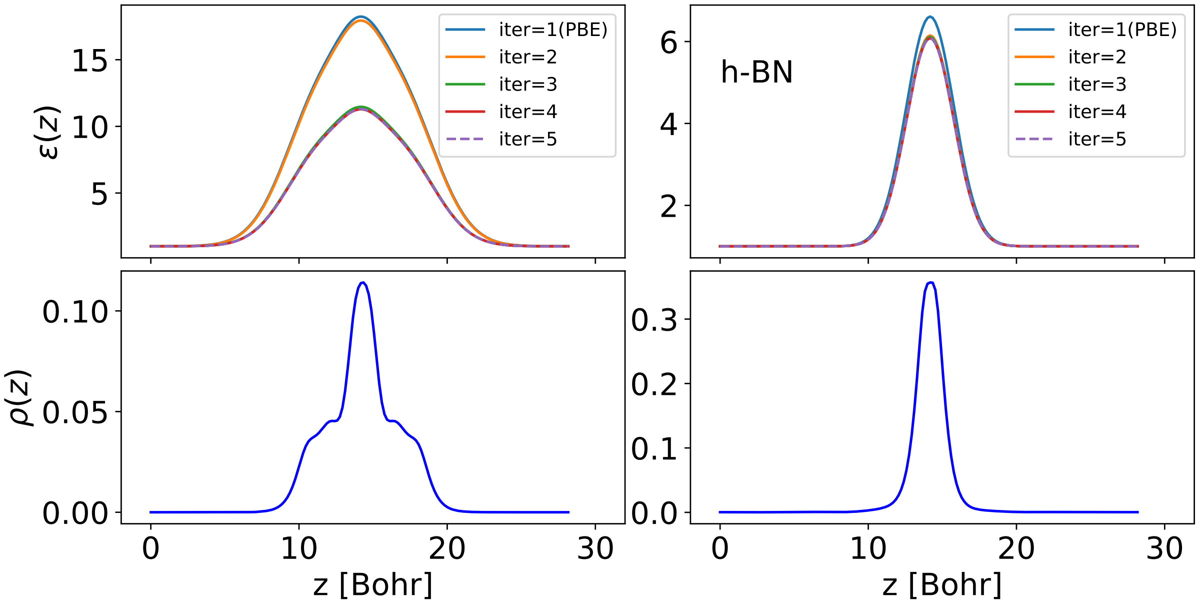


FIG. S 3. Local dielectric function $\epsilon(z)$ (Upper panels) and charge density $\rho(z)$ (Lower panels) (in unit of e/Bohr$^3$) for $MoS_2$ and h-BN. $MoS_2$ and h-BN are located on a XY plane at $z =\sim 14$ Bohr.

## IV. ANALYSIS OF FINITE-SIZE EFFECTS AND CHOICE OF PSEUDOPOTENTIAL

### A. Finite-size effects

All of our calculations were performed using supercells, using the Γ point to sample the Brillouin zone and the number of atoms shown in Table I.

TABLE I. Number of atoms in the supercell

| Systems | Si | SiC | AlP | Diamond | MgO | LiCl | Ar | Ne |
|---|---|---|---|---|---|---|---|---|
| No. of atoms | 512 | 512 | 128 | 512 | 128 | 64 | 32 | 32 |

In Table II we compare the PBE band gaps computed from supercell calculations with those obtained using unit cells and different k-point samplings, and the same pseudopotential (ONCV).The calculations on unit cell were performed using Quantum Espresso [9, 10]. The results of the table show that finite size effects on the band gaps computed with the supercells used in the main text are negligible.

TABLE II. PBE band gap (eV) for bulk systems: energy cutoff 70Ry

| | $8 \times 8 \times 8$ | $16 \times 16 \times 16$ | Supercell |
|---|---|---|---|
| AlP | 1.572 | 1.572 | 1.560 |
| Diamond | 4.175 | 4.175 | 4.175 |
| MgO | 4.783 | 4.783 | 4.778 |
| LiCl | 6.474 | 6.471 | 6.469 |
| Ar | 6.701 | 6.701 | 6.702 |
| Ne | 11.617 | 11.617 | 11.616 |

### B. Choice of pseudopotential

We compare the results for the band gaps of three-dimensional solids, at the PBE level, obtained with ONCV and MT_FHI pseudopotentials; the latter were used to carry out calculations with Quantum Espresso in Ref. [11]. We observed differences in the range 0.05 - 0.15 eV. We observed differences up to 0.2 eV when comparing pseudopotential (PP) calculations with the all-electron (AE) results of Ref. [11]. These differences may in partly arise from the different basis sets in PP and AE calculations. We also note that we observed additional differences when using different pseudopotentials and using DDH functionals. For example: for Ne, DDH calculations ($\alpha = 1/\epsilon_\infty$) with the ONCV pseudopotential gives a band gap of 22.67 eV, whereas those the with MT_FHI pseudopotential gives a value of 23.36 (in this case we set $\epsilon_\infty$ to be 1.21). The DDH band gap from Ref. [11] is 23.67 eV ($\epsilon_\infty = 1.21$).

TABLE III. PBE gaps computed using different pseudopotentials

| | Qbox(ONCV [a]) | QE (MT_FHI) | Ref. [11] |
|---|---|---|---|
| AlP | 1.560 | 1.582 | 1.64 |
| Diamond | 4.175 | 4.245 | 4.15 |
| MgO | 4.778 | 4.607 | 4.80 |
| LiCl | 6.469 | 6.431 | 6.54 |
| Ar | 8.700 | 8.653 | 8.78 |
| Ne | 11.616 | 11.569 | 11.65 |

[a] Version 1.2 of ONCV was used for Ar, and Version 1.0 were used for the other solids. ONCV 1.0 and ONCV 1.2 give same results for all the systems except Ar.


[1] D. R. Hamann, Phys. Rev. B **88**, 085117 (2013).
[2] M. Schlipf and F. Gygi, Computer Physics Communications **196**, 36 (2015).
[3] F. Gygi, `http://www.quantum-simulation.org/potentials/sg15_oncv/` (Accessed December 12, 2018).
[4] F. Gygi, `http://qboxcode.org/trac/wiki/SiC512` (Accessed December 12, 2018).
[5] T. A. Pham, D. Lee, E. Schwegler, and G. Galli, Journal of the American Chemical Society **136**, 17071 (2014).
[6] T. Anh Pham, T. Li, H.-V. Nguyen, S. Shankar, F. Gygi, and G. Galli, Applied Physics Letters **102**, 241603 (2013).
[7] `https://materialsproject.org/` (Accessed December 12, 2018).

[8] "The general properties of Si, Ge, SiGe, SiO2 and Si3N4," `http://www.virginiasemi.com/pdf/generalpropertiesSi62002.pdf` (2002).

[9] P. Giannozzi, S. Baroni, N. Bonini, M. Calandra, R. Car, C. Cavazzoni, D. Ceresoli, G. L. Chiarotti, M. Cococcioni, I. Dabo, A. Dal Corso, S. de Gironcoli, S. Fabris, G. Fratesi, R. Gebauer, U. Gerstmann, C. Gougoussis, A. Kokalj, M. Lazzeri, L. Martin-Samos, N. Marzari, F. Mauri, R. Mazzarello, S. Paolini, A. Pasquarello, L. Paulatto, C. Sbraccia, S. Scandolo, G. Sclauzero, A. P. Seitsonen, A. Smogunov, P. Umari, and R. M. Wentzcovitch, Journal of Physics: Condensed Matter **21**, 395502 (19pp) (2009).

[10] P. Giannozzi, O. Andreussi, T. Brumme, O. Bunau, M. B. Nardelli, M. Calandra, R. Car, C. Cavazzoni, D. Ceresoli, M. Cococcioni, N. Colonna, I. Carnimeo, A. D. Corso, S. de Gironcoli, P. Delugas, R. A. D. Jr, A. Ferretti, A. Floris, G. Fratesi, G. Fugallo, R. Gebauer, U. Gerstmann, F. Giustino, T. Gorni, J. Jia, M. Kawamura, H.-Y. Ko, A. Kokalj, E. Küçükbenli, M. Lazzeri, M. Marsili, N. Marzari, F. Mauri, N. L. Nguyen, H.-V. Nguyen, A. O. de-la Roza, L. Paulatto, S. Poncé, D. Rocca, R. Sabatini, B. Santra, M. Schlipf, A. P. Seitsonen, A. Smogunov, I. Timrov, T. Thonhauser, P. Umari, N. Vast, X. Wu, and S. Baroni, Journal of Physics: Condensed Matter **29**, 465901 (2017).

[11] J. H. Skone, M. Govoni, and G. Galli, Phys. Rev. B **89**, 195112 (2014).
